# Supplementary material for: GIVEPose: Gradual Intra-class Variation Elimination for RGB-based Category-Level Object Pose Estimation
Source: arXiv:2503.15110 source file (2025-03-20)
Supplement: Supplementary file 1 [file X_suppl.tex]

\clearpage
\setcounter{page}{1}

\setcounter{figure}{0} 
\setcounter{table}{0}
\setcounter{equation}{0}

% \maketitlesupplementary
\maketitle

\appendix
% \addcontentsline{toc}{section}{Appendix}
{
% % \begingroup
\color{red}
\hypersetup{linkcolor=red}
\tableofcontents
% \endgroup
}

\section{More Details of Loss Functions}
As shown in Sec.~3.5 of the main paper, our overall loss function consists of three components: $L_{pose}$, $L_{nocs}$, and $L_{ivfc}$. Here, we present the detailed formulation of each loss term.

\subsection{Pose losses}
Following LaPose~\cite{zhang2024lapose}, we employ similar loss functions to supervise pose regression. 
The overall pose loss is 
\begin{equation}
\begin{aligned}
L_{pose} =&~\omega_{rot}L_{rot} + \omega_{pm}L_{pm} \\
           &~+\omega_{trans}L_{trans} + \omega_{size}L_{size},
 \label{eq:pose_loss}
 \end{aligned}
\end{equation}
where $\omega_{rot}$, $\omega_{pm}$, $\omega_{trans}$, and $\omega_{size}$ are the weighting hyper-parameters. 

Specifically, $L_{trans}$ and $L_{size}$ are utilized to supervise the scale-agnostic translation and size, respectively:

\begin{equation}
\begin{split}
    L_{trans} &= \|\hat{t} - t_{gt}\|_1, \\
    L_{size} &= \|\hat{s} - s_{gt}\|_1,
\end{split}   
\end{equation}
where $\hat{t}$ and $\hat{s}$ represent the predicted scale-agnostic translation and size respectively, $t_{gt}$ and $s_{gt}$ denote corresponding ground truth value.

Both $L_{rot}$ and $L_{pm}$ serve as supervision terms for rotation learning, where $L_{rot}$ directly supervises the rotation matrix, and the point matching loss $L_{pm}$~\cite{wang2021gdr} is calculated by first applying rotational transformations to the points on the model:

\begin{equation}
\begin{aligned}
        & L_{rot} = \|\hat{R} - R_{gt}\|_1,    \\
        & L_{pm} = \text{avg}_{x \in \mathbf{M}}\| \hat{R} x - R_{gt} x\|_1, 
\end{aligned}
\end{equation}
where $R_{gt}$ represents the ground-truth rotation matrix for supervising the predicted $\hat{R}$, and $x$ denotes the sampled points from the object's NOCS model $\mathbf{M}$. 
To handle ambiguous rotations arising from object symmetry~\cite{pitteri2019sym}, we supervise the prediction using the closest rotation selected from the proper symmetry group for symmetrical categories.

\subsection{Geometric losses in GIVE}
For the implementation of our proposed GIVE strategy, we utilize $L_{nocs}$ and $L_{ivfc}$ to supervise two intermediate representations, the NOCS map and the IVFC map:

\begin{equation}
    L_{nocs} = \|M_{nocs} \cdot (N^{gt}_{map} - \hat{N}_{map})\|_1,
\end{equation}
where $M_{nocs}$ represents the mask of the NOCS map and the $N^{gt}_{map}$ is the supervision of predicted NOCS map $\hat{N}_{map}$.

\begin{equation}
    L_{ivfc} = \|M_{ivfc} \cdot (C^{gt}_{map} - \hat{C}_{map})\|_1,
\end{equation}
where $M_{ivfc}$ denotes the mask of the IVFC map and the prediction of IVFC map $\hat{C}_{map}$ is supervised by corresponding ground-truth value $C^{gt}_{map}$.

\begin{figure*}[t]
  \centering
   \includegraphics[width=0.75\linewidth]{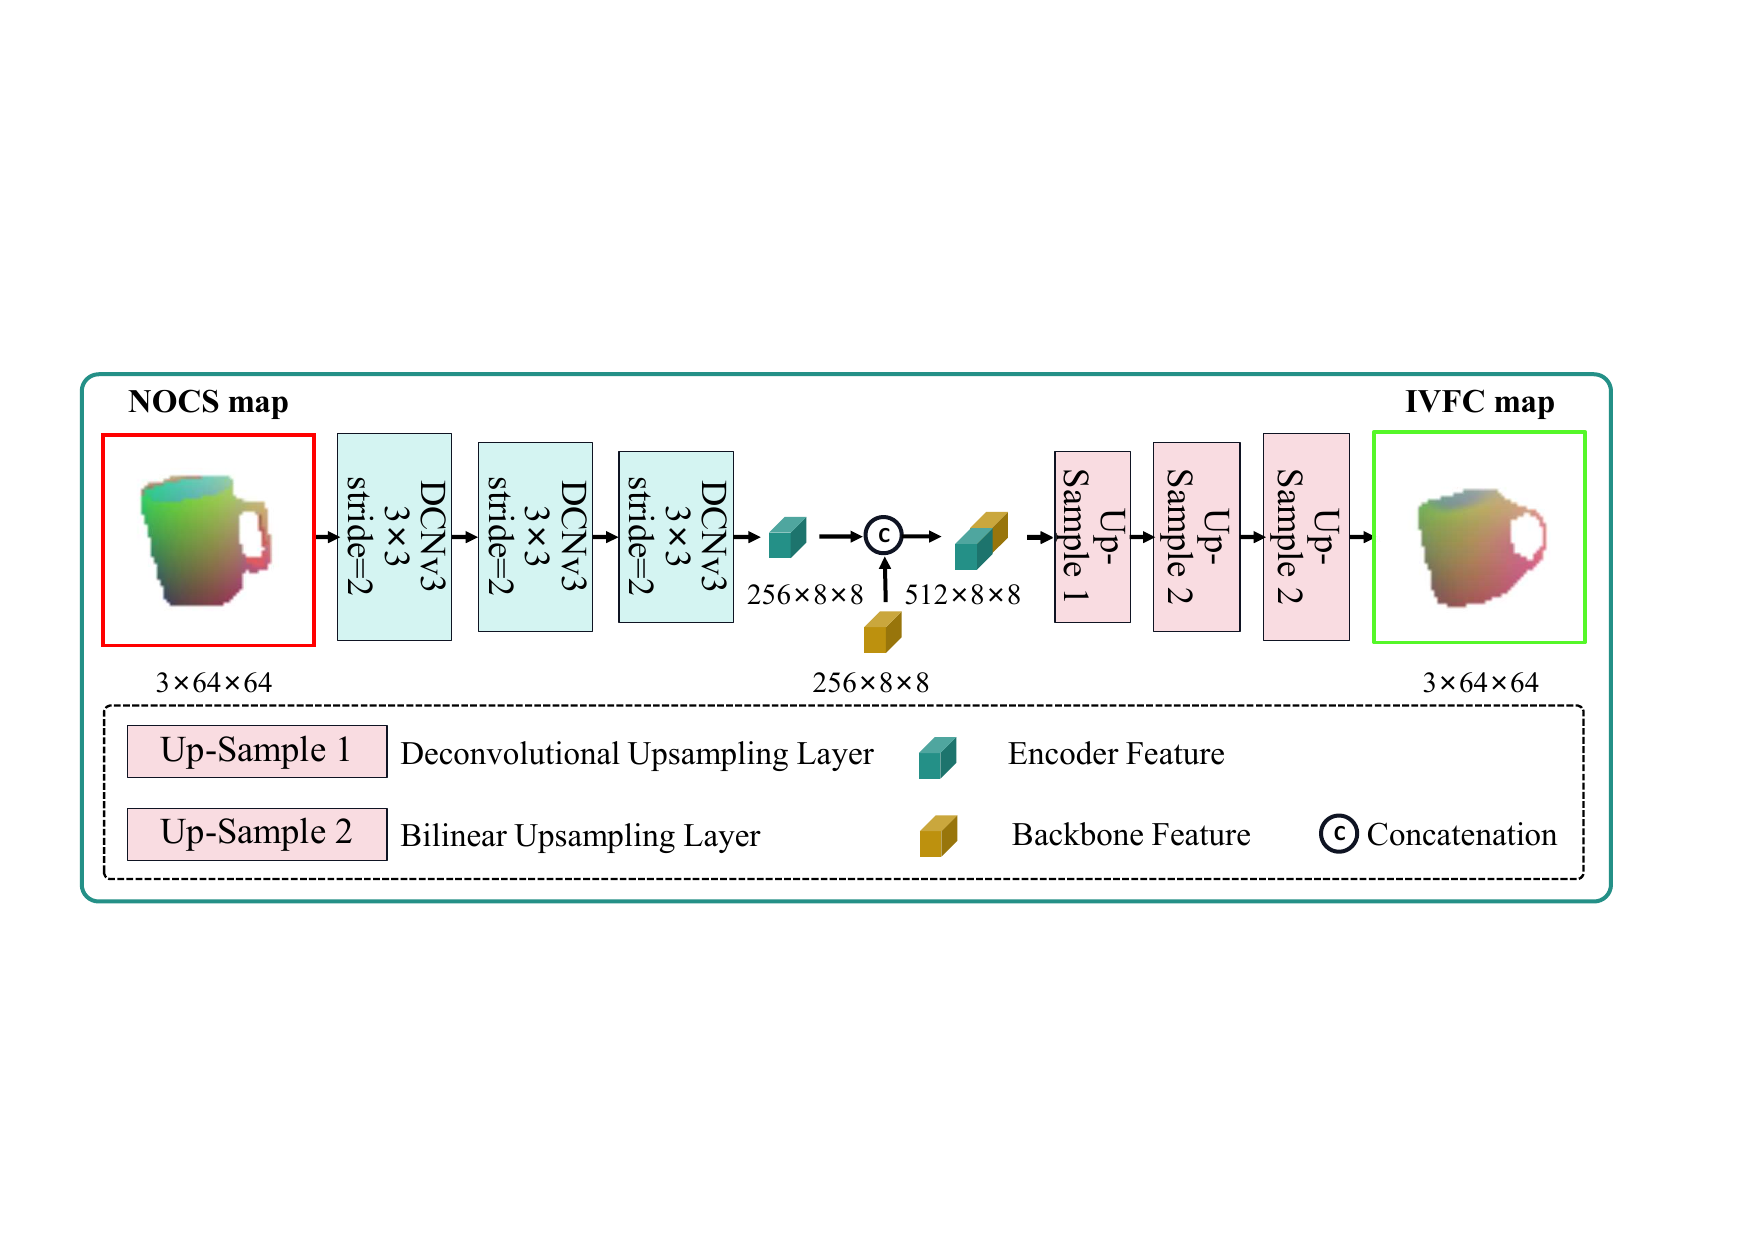}
   \caption{Detailed structural diagram of the Deformable Convolutional Auto-Encoder (DCAE)-based module.
   }
   \label{fig:dcae}
\end{figure*}

\section{Details of Deformable Convolutional Auto-Encoder (DCAE)-based module}

Throughout the network architecture, the DCAE-based module serves as the key component for achieving gradual intra-class variation elimination. 

In our implementation, we adopt the deformable convolution (specifically, DCNv3) proposed in \cite{wang2023dcnv3}. 
As illustrated in \cref{fig:dcae}, we employ three layers of deformable convolutions with a stride of 2 to extract features and reduce the resolution from the predicted NOCS map, resulting in a feature map of size \(256\times8\times8\). 
Compared to vanilla convolutions, deformable convolutions feature adaptable convolution kernels, enabling more flexible spatial correspondence between feature maps and input coordinate maps. 
This flexibility allows for a more robust capture of category-consensus information from the NOCS map. 
The extracted features are subsequently concatenated with backbone features. 
Finally, the concatenated feature map undergoes three upsampling operations, consisting of one deconvolution and two bilinear interpolations, to generate the IVFC map with redundant instance information eliminated.

\section{Details of Category-Consensus Model Reconstruction}

As mentioned in Sec.~4.2 of the main paper, to obtain the mesh models for generating IVFC maps, we performed surface reconstruction on per-category mean point cloud models using functions from the Open3D~\cite{zhou2018open3d} library. Specifically, we first reconstructed mesh models directly from point clouds using the \textbf{$create\_from\_point\_cloud\_alpha\_shape$} function, followed by applying Laplacian smoothing through the \textbf{$filter\_smooth\_laplacian$} function. Following the approach in NOCS~\cite{zhang2024lapose}, we further color-coded the mesh models based on their coordinate values to obtain the color-coded category-consensus model, as shown in \cref{fig:vis_model}.

\begin{figure}[b]
  \centering
   \includegraphics[width=0.8\linewidth]{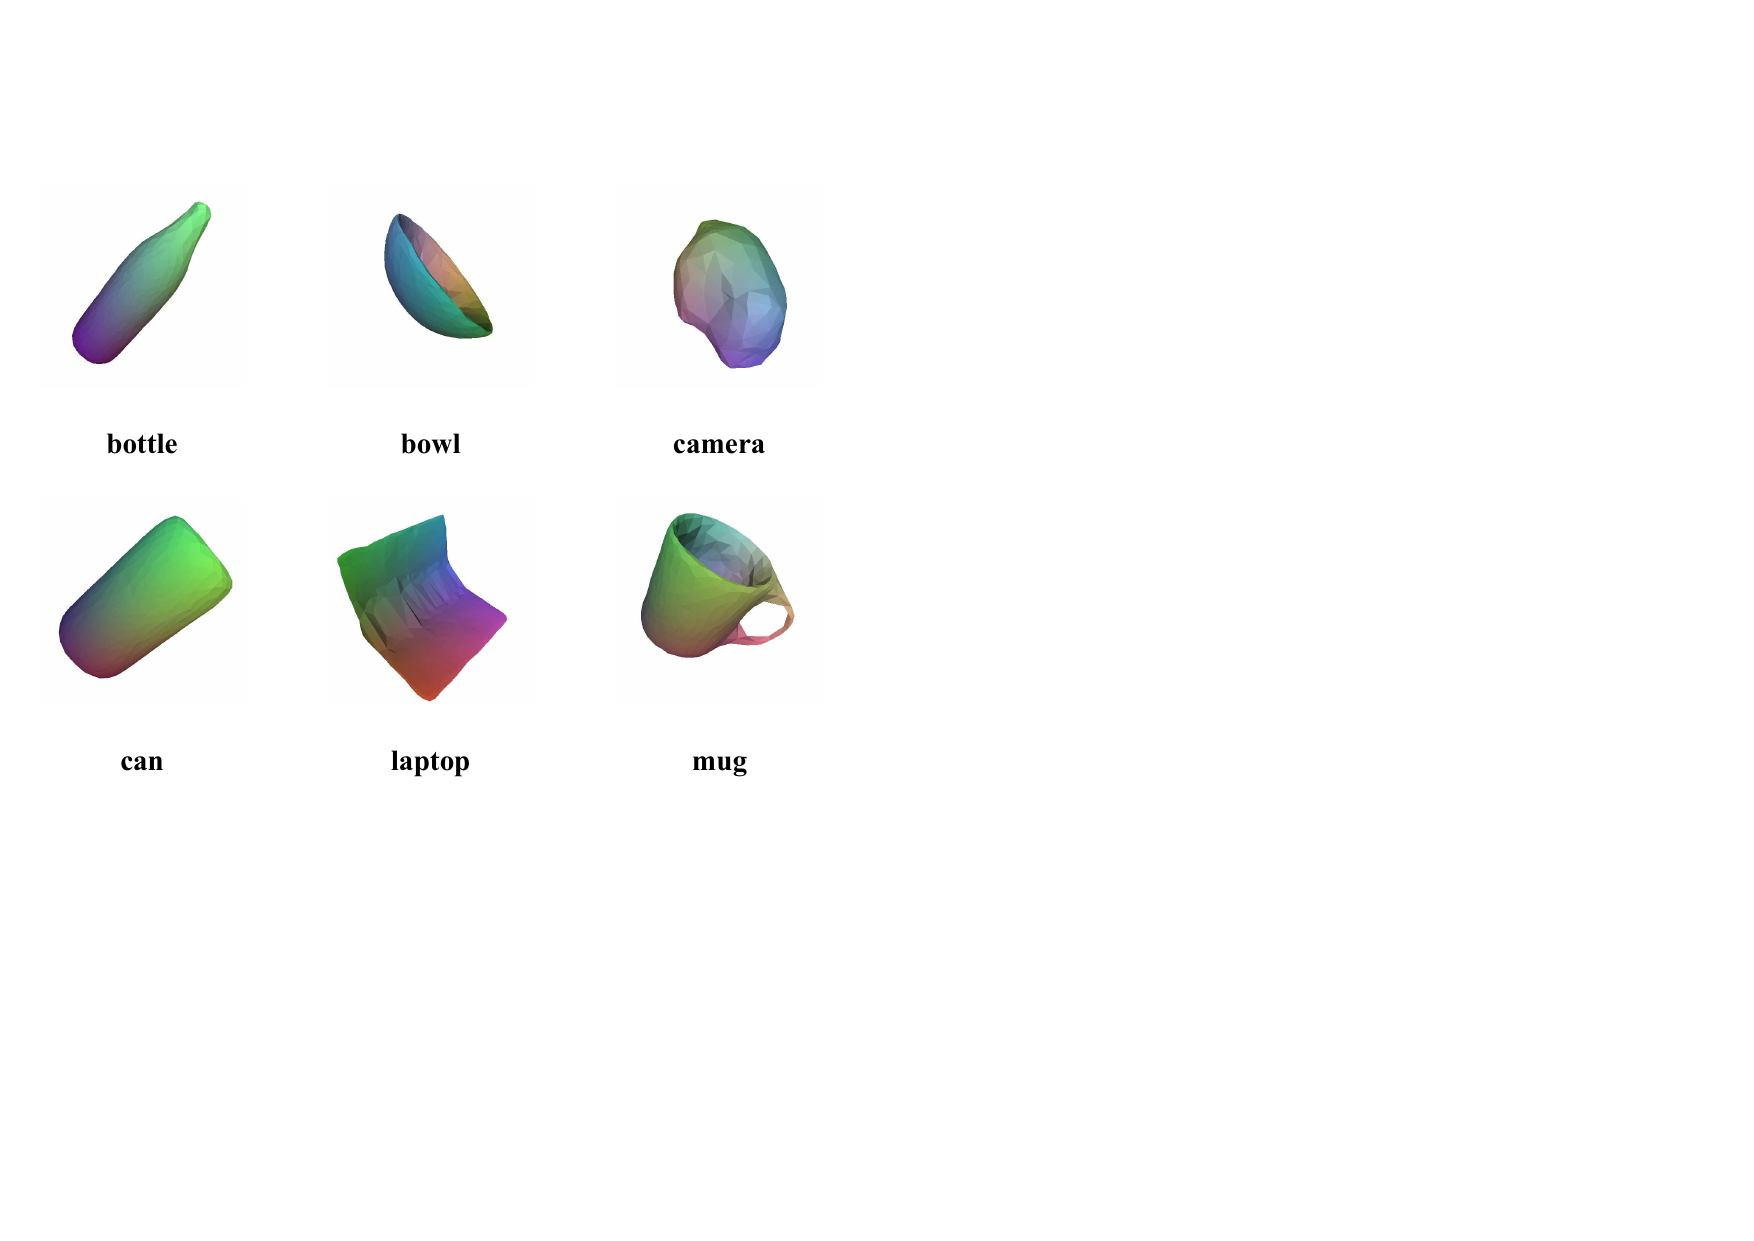}
   \caption{Color-coded consensus models for each category.
   }
   \label{fig:vis_model}
\end{figure}

\section{Extended Quantitative Evaluation}
\subsection{Per-category results}
\cref{tab:real_percat}, \cref{tab:camera_percat}, and \cref{tab:wild_percat} present the detailed evaluation results of our GIVEPose for each category on REAL275, CAMERA25 \cite{wang2019normalized}, and Wild6D \cite{fu2022wild6d} datasets using scale-agnostic evaluation metrics \cite{zhang2024lapose}.

\begin{figure}[t]
  \centering
   \includegraphics[width=0.85\linewidth]{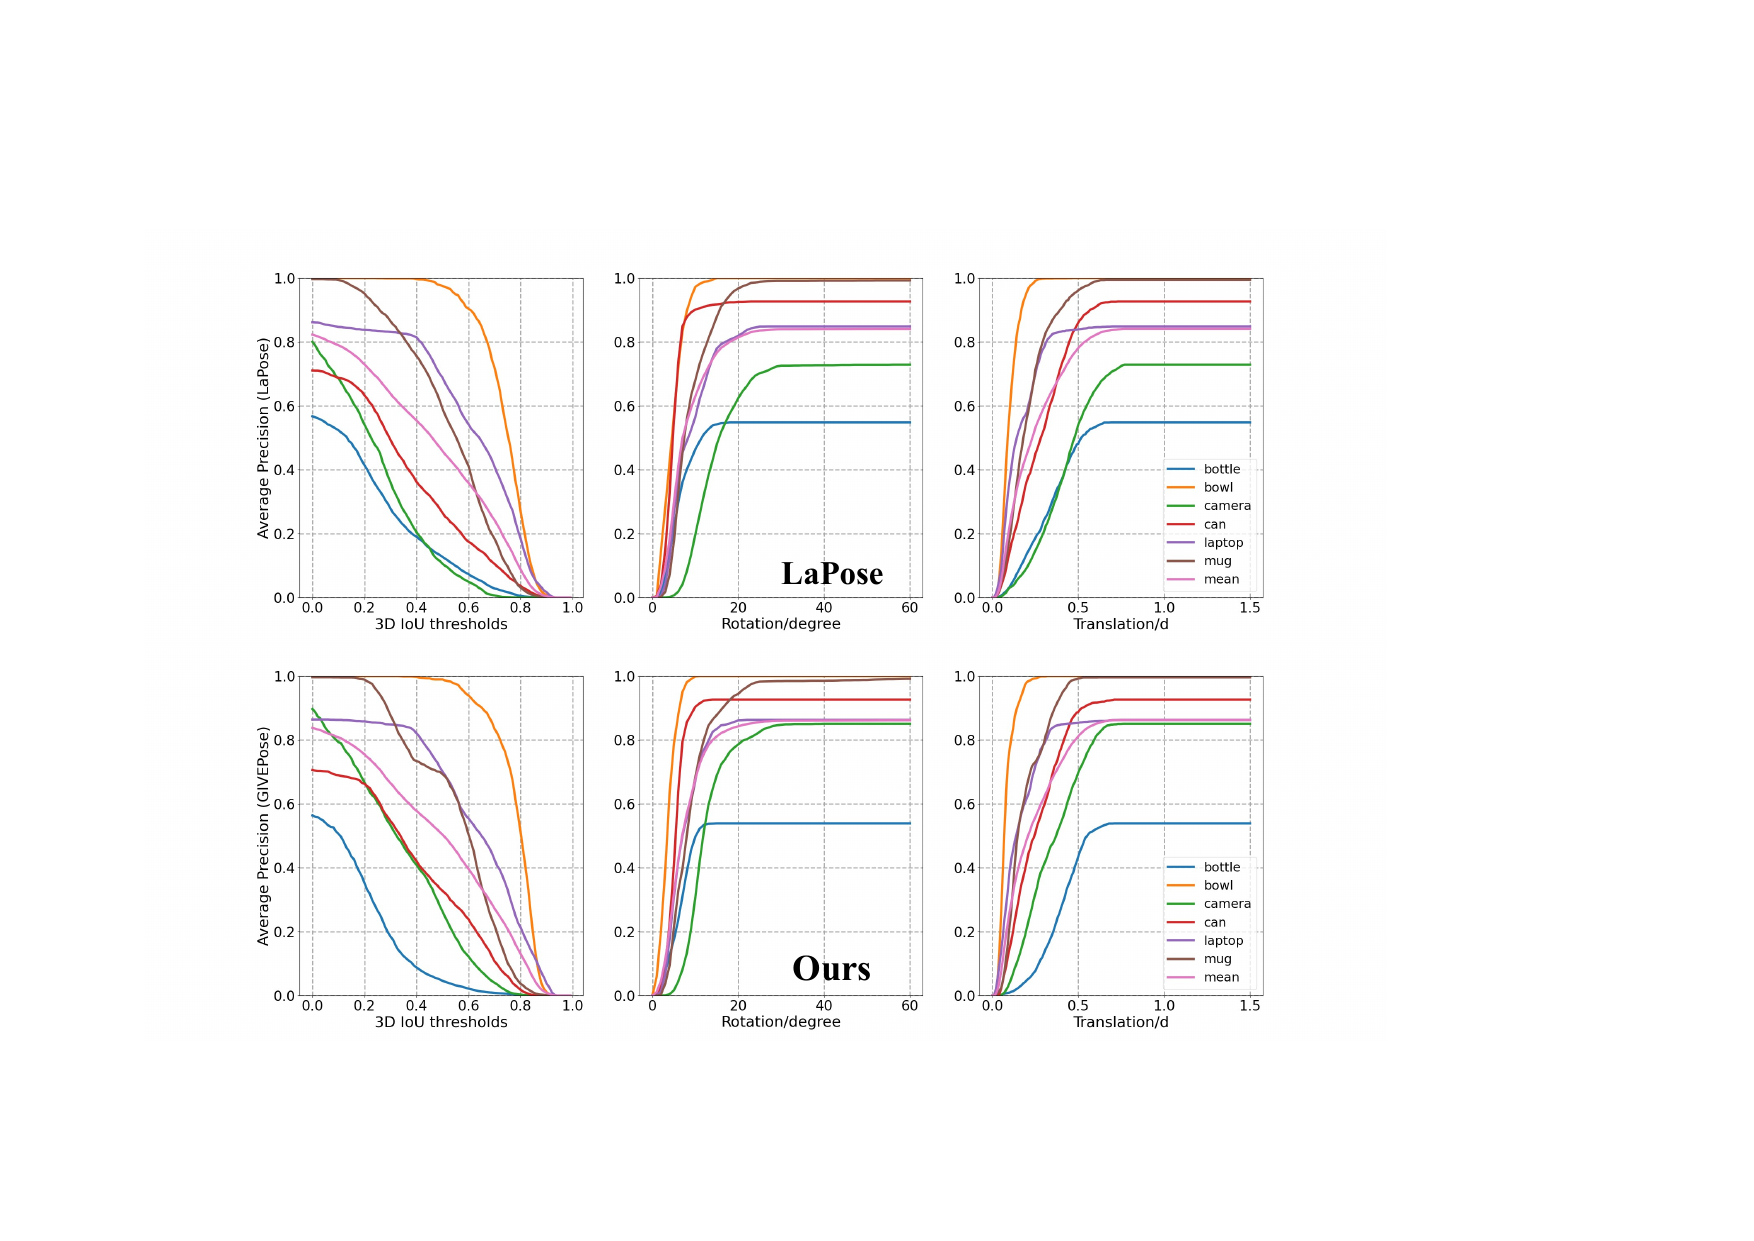}
   \caption{Detailed Comparison with Lapose~\cite{zhang2024lapose} on the REAL275 dataset using scale-agnostic evaluation metrics.}
   \label{fig:percat_comp}
\end{figure}

\subsection{Detailed Performance Comparison of Our Method against LaPose}
For a more detailed comparison with existing methods, we provide per-category results of our method and LaPose~\cite{zhang2024lapose} in \cref{fig:percat_comp}. As illustrated in the figure, our method shows significant improvements over LaPose~\cite{zhang2024lapose} for categories with large intra-class variation (e.g., camera), which can be attributed to our gradual intra-class variation elimination strategy. For the bottle category, our method experiences a slight performance drop, which we attribute to the joint training of multiple categories, where inter-category influences may occur. Overall, our method outperforms LaPose~\cite{zhang2024lapose}, achieving better average results and superior performance across most categories, thereby demonstrating its effectiveness.

\begin{table*}[b]
    \centering
    \tablestyle{16pt}{1.1}
    \begin{tabular}{@{}l|c c c|c c c c c@{}}
    % \toprule
        Category & $NIoU_{25}$ & $NIoU_{50}$ & $NIoU_{75}$ & $10^\circ 0.2d$ & $10^\circ 0.5d$ & $0.2d$ & $0.5d$ & $10^\circ$ \\ 
        \shline
        bottle & 26.6 & 4.6 & 0.5 & 4.6 & 39.6 & 4.8 & 43.5 & 49.7 \\ 
        bowl   & 100.0 & 98.9 & 73.5 & 97.9 & 99.9 & 98.1 & 100.0 & 99.9 \\
        camera & 60.2 & 26.3 & 1.3 & 10.2 & 27.8 & 21.1 & 69.8 & 30.8 \\ 
        can   & 61.3 & 32.8 & 6.1 & 41.7 & 86.7 & 41.9 & 88.7 & 90.4 \\ 
        laptop & 85.4 & 70.2 & 33.2 & 56.6 & 66.6 & 61.8 & 85.4 & 67.2 \\ 
        mug  & 95.1 & 69.3 & 10.2 & 56.7 & 68.5 & 65.8 & 99.2 & 68.5 \\
        \hline
        average &71.4 & 50.3& 20.8 & 44.6 & 64.8 & 48.9 & 81.1 & 67.8 \\
        % \bottomrule
    \end{tabular}    \caption{\label{tab:real_percat}Per-category results on the REAL275 dataset using scale-agnostic evaluation metrics.}    
\end{table*}
\begin{table*}[b]
    \centering
    \tablestyle{16pt}{1.1}
    \begin{tabular}{@{}l|c c c|c c c c c@{}}
    % \toprule
        Category & $NIoU_{25}$ & $NIoU_{50}$ & $NIoU_{75}$ & $10^\circ 0.2d$ & $10^\circ 0.5d$ & $0.2d$ & $0.5d$ & $10^\circ$ \\ 
        \shline
        bottle & 78.0 & 57.6 & 20.4 & 56.1 & 82.6 & 56.2 & 83.2 & 87.4 \\ 
        bowl   & 95.4 & 86.7 & 35.6 & 82.5 & 95.6 & 82.9 & 96.3 & 95.9 \\
        camera & 60.0 & 23.9 & 3.3 & 18.1 & 59.9 & 21.5 & 72.6 & 72.2 \\ 
        can   & 76.5 & 52.1 & 13.4 & 43.6 & 78.5 & 43.6 & 78.5 & 87.2 \\ 
        laptop & 92.1 & 74.8 & 39.3 & 68.2 & 89.5 & 72.0 & 95.6 & 91.7 \\ 
        mug  & 54.8 & 24.8 & 4.2 & 16.3 & 7.2 & 22.1 & 64.1 & 59.8 \\
        \hline
        average &76.1 & 53.3& 19.4 & 47.5 & 75.5 & 82.4 & 49.7 & 81.7 \\ 
        % \bottomrule
    \end{tabular}    
    \caption{
    \label{tab:camera_percat}
    Per-category results on the CAMERA25 dataset \cite{wang2019normalized} using scale-agnostic evaluation metrics.}    
\end{table*}
\begin{table*}[b]
    \centering
    \tablestyle{16pt}{1.1}
    \begin{tabular}{@{}l|c c c|c c c c c@{}}
    % \toprule
        Category & $NIoU_{25}$ & $NIoU_{50}$ & $NIoU_{75}$ & $10^\circ 0.2d$ & $10^\circ 0.5d$ & $0.2d$ & $0.5d$ & $10^\circ$ \\ 
        \shline
        bottle & 87.3 & 62.4 & 17.4 & 57.1 & 76.7 & 68.9 & 94.9 & 77.3 \\ 
        bowl   & 99.3 & 91.8 & 42.9 & 87 & 96.2 & 88.5 & 99.7 & 96.3 \\
        camera & 60.8 & 22.0 & 0.3 & 1.2 & 2.8 & 26.4 & 73.4 & 3.0 \\ 
        laptop & 99.7 & 99.6 & 79.9 & 18 & 18.1 & 99.4 & 99.7 & 18.1 \\ 
        mug  & 89.6 & 26.4 & 0.1 & 3.9 & 7.5 & 24 & 93.7 & 7.5 \\
        \hline
        average &87.3 & 60.4& 28.1 & 33.4 & 40.3 & 61.4 & 92.3 & 40.4\\
        % \bottomrule
    \end{tabular}    
    \caption{\label{tab:wild_percat}
    Per-category results on the Wild6D dataset \cite{fu2022wild6d} using scale-agnostic evaluation metrics.}    
\end{table*}

\section{Extended Qualitative Analysis}
To facilitate a more comprehensive and intuitive evaluation, we present extended qualitative comparisons between our approach and four existing methods~\cite{lee2021category, lin2022category, wei2023rgb,zhang2024lapose} in \cref{fig:real_vis_sup} and \cref{fig:camera_vis_sup}. 
These results demonstrate that our method achieves more accurate category-level pose estimation compared to existing approaches, particularly when handling categories with large intra-class variations and processing truncated cropped images.

\section{Code and Reproducibility}
We provide our PyTorch-based~\cite{paszke2019pytorch} code in the ``GIVEPOSE'' folder for anonymous review, with detailed instructions for reproducing experimental results available in the ``GIVEPOSE/README.md'' file. 
The code will be publicly released upon acceptance.

\section{Ethics Statement}
Despite the consideration of scene and object diversity in the publicly available datasets we used, potential biases continue to exist. We acknowledge the significant computational resources and energy consumption required for training and inference, which could raise environmental concerns. Efforts are being made to minimize these impacts through efficient computation strategies and exploring more sustainable AI practices. Furthermore, all datasets were used in compliance with ethical standards, ensuring data privacy.

\begin{figure*}[t]
\centering
\includegraphics[width=0.8\textwidth]{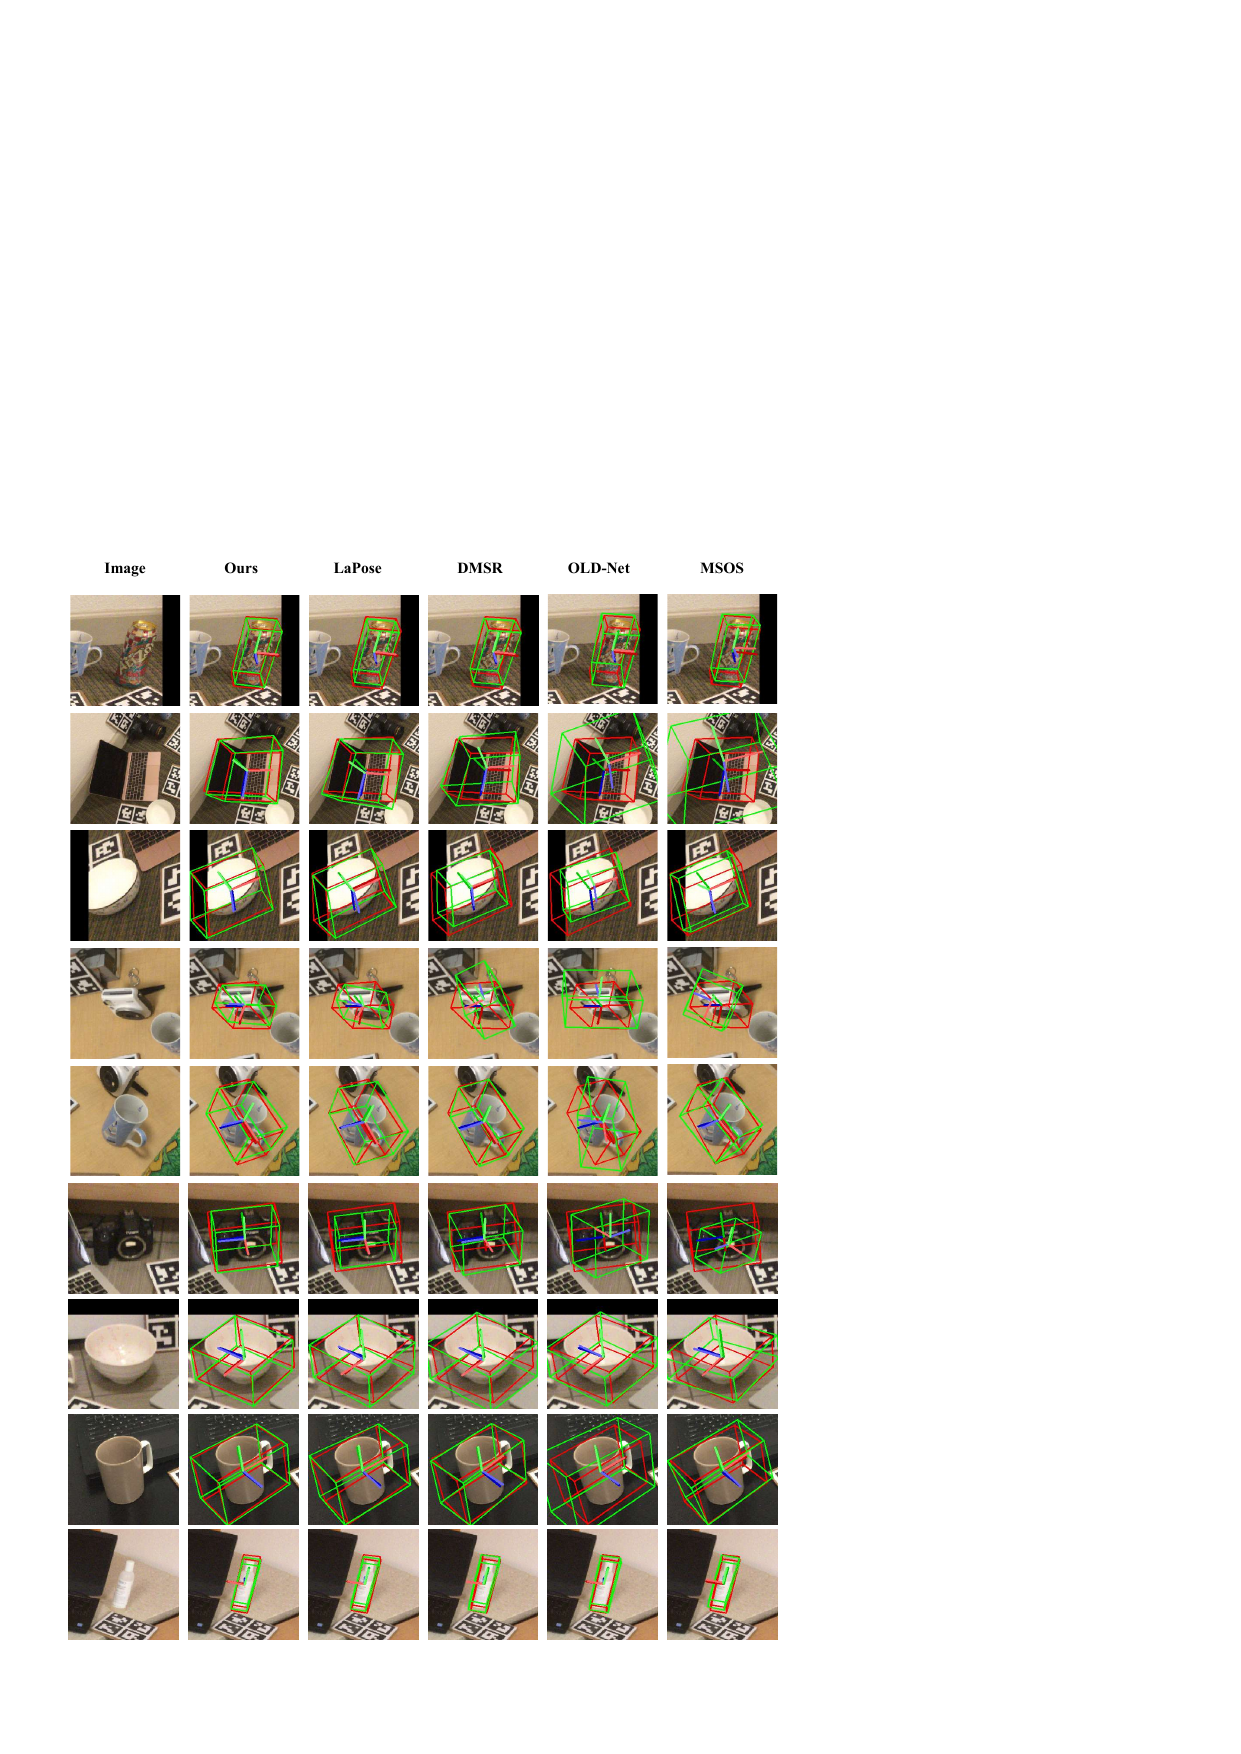}
\caption{Qualitative comparisons on \textbf{REAL275}. 
For the 3D box visualization, \textcolor{red}{red} denotes the ground truth and \textcolor{green}{green} represents the predicted result. 
For the axis projections, darker shades indicate the ground truth, while lighter shades correspond to the predicted results.
}
\label{fig:real_vis_sup}
\end{figure*}

\begin{figure*}[t]
\centering
\includegraphics[width=0.8\textwidth]{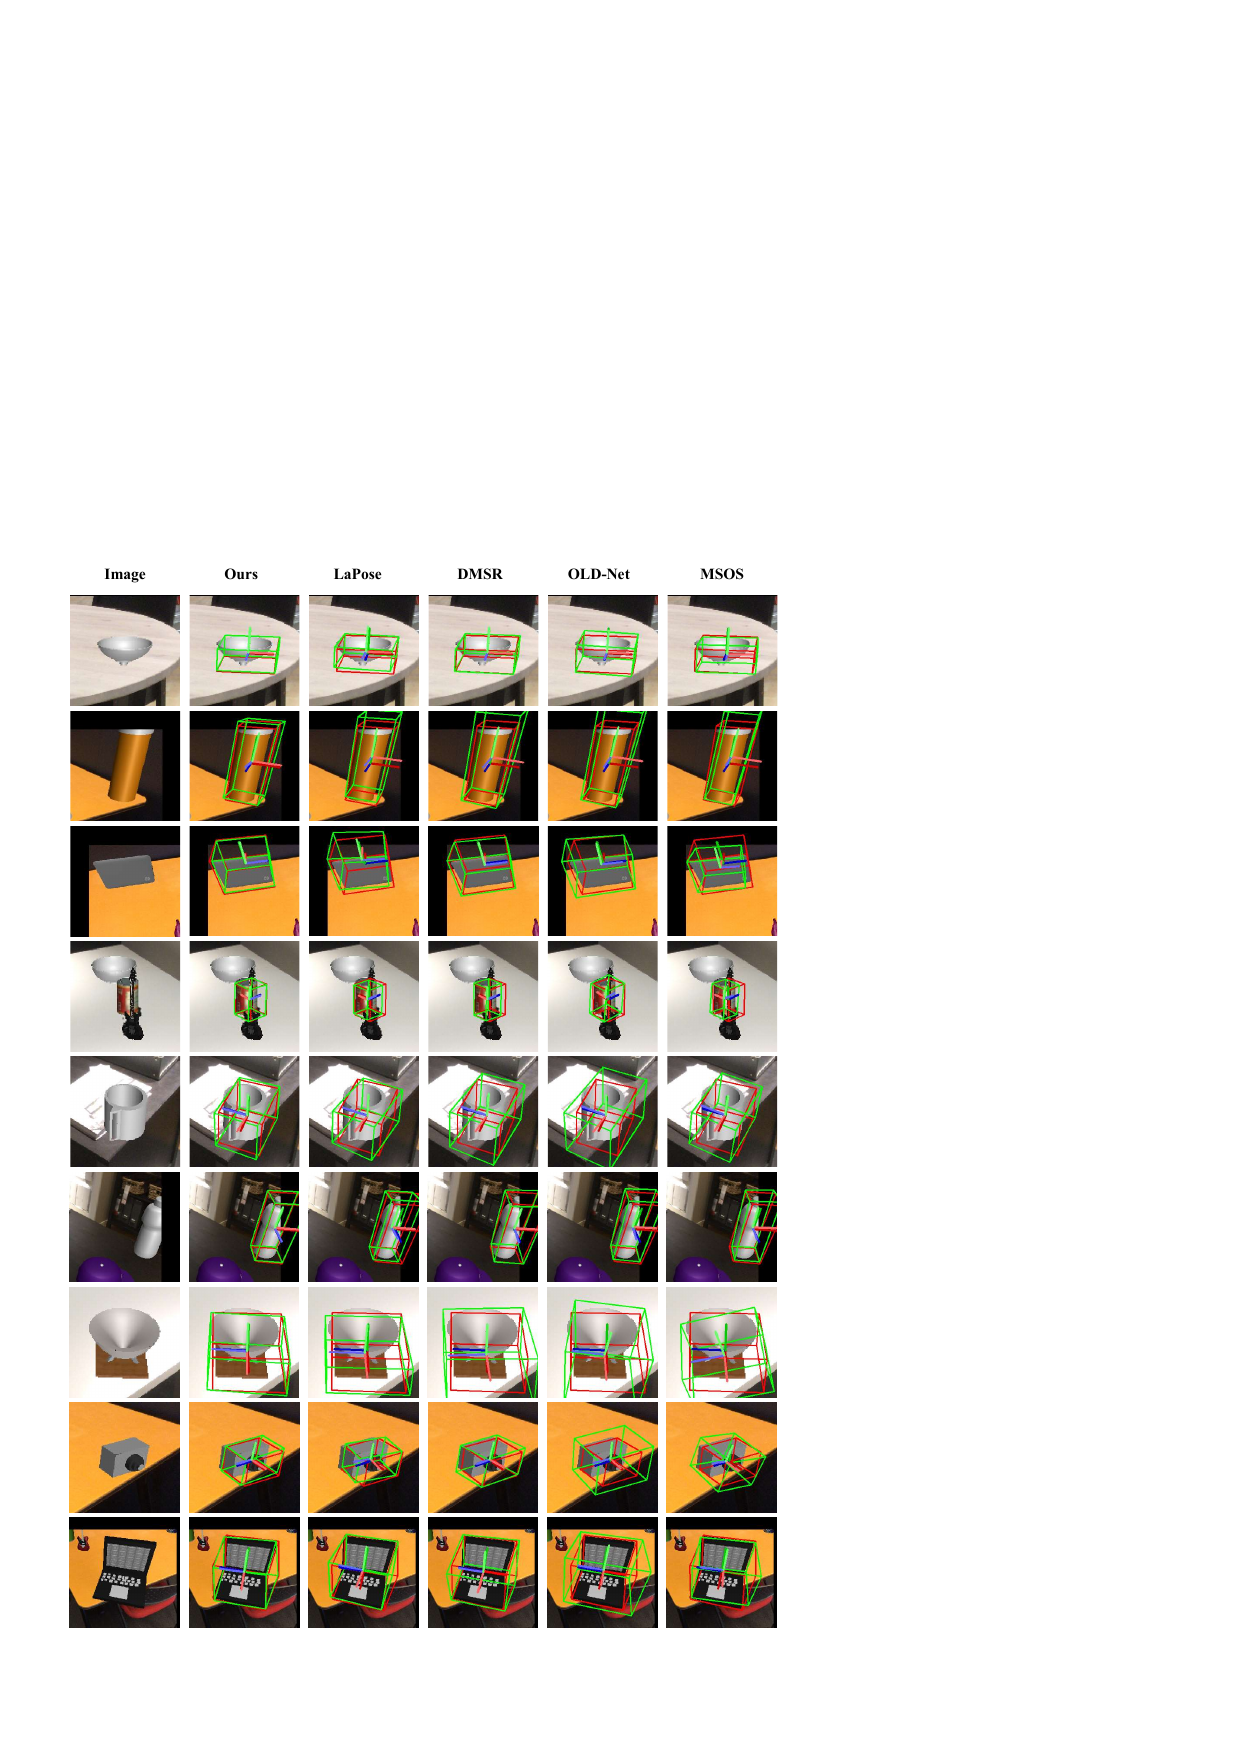}
\caption{Qualitative comparisons on \textbf{CAMERA25}. For the 3D box visualization, \textcolor{red}{red} denotes the ground truth and \textcolor{green}{green} represents the predicted result. 
For the axis projections, darker shades indicate the ground truth, while lighter shades correspond to the predicted results.
}
\label{fig:camera_vis_sup}
\end{figure*}

% \section{Rationale}
% \label{sec:rationale}
% % 
% Having the supplementary compiled together with the main paper means that:
% % 
% \begin{itemize}
% \item The supplementary can back-reference sections of the main paper, for example, we can refer to \cref{sec:intro};
% \item The main paper can forward reference sub-sections within the supplementary explicitly (e.g. referring to a particular experiment); 
% \item When submitted to arXiv, the supplementary will already included at the end of the paper.
% \end{itemize}
% % 
% To split the supplementary pages from the main paper, you can use \href{https://support.apple.com/en-ca/guide/preview/prvw11793/mac#:~:text=Delete%20a%20page%20from%20a,or%20choose%20Edit%20%3E%20Delete).}{Preview (on macOS)}, \href{https://www.adobe.com/acrobat/how-to/delete-pages-from-pdf.html#:~:text=Choose%20%E2%80%9CTools%E2%80%9D%20%3E%20%E2%80%9COrganize,or%20pages%20from%20the%20file.}{Adobe Acrobat} (on all OSs), as well as \href{https://superuser.com/questions/517986/is-it-possible-to-delete-some-pages-of-a-pdf-document}{command line tools}.
